# Supplementary material for: Unconventional Superconductivity in Magic-Angle Twisted Trilayer Graphene
Source: arXiv:2104.10176 source file (2022-01-14)
Supplement: Supplementary file 1 [file supp.pdf]

# Supplemental Material
# Unconventional Superconductivity in Magic-Angle Twisted Trilayer Graphene


Ammon Fischer,[1] Zachary A. H. Goodwin,[2] Arash Mostofi,[2]
Johannes Lischner,[2] Dante M. Kennes,[1,3,*] and Lennart Klebl[1,†]

[1]*Institute for Theory of Statistical Physics, RWTH Aachen University, and JARA Fundamentals of Future Information Technology, 52062 Aachen, Germany*
[2]*Departments of Materials and Physics and the Thomas Young Centre for Theory and Simulation of Materials, Imperial College London, South Kensington Campus, London SW7 2AZ, UK*
[3]*Max Planck Institute for the Structure and Dynamics of Matter, Center for Free Electron Laser Science, 22761 Hamburg, Germany*



(Dated: January 14, 2022)


## SUPPLEMENTARY METHODS

*Structural Relaxations* In Fig. 1 we display the out-of-plane corrugation that occurs upon relaxing MATTG at 1.61°. At this angle, which is close to the magic angle of TTG, the $z$-displacements exhibit the largest effects as the unit cells are not large enough for significant in-plane relaxations to occur [1]. We find that the inner, twisted layer essentially does not undergo any out-of-plane relaxations. The outer layers undergo significant relaxations to minimise the energy of the structure. In the AAA regions of the moiré unit cell (corners of the plot), an interlayer spacing of almost 3.6 Å is reached; whereas in the ABA (or ACA) regions of the moiŕe unit cell, the interlayer spacing is closer to 3.35 Å. These interlayer spacings reflect the equilibrium bilayer stacking of AA and AB bilayer graphene, respectively.

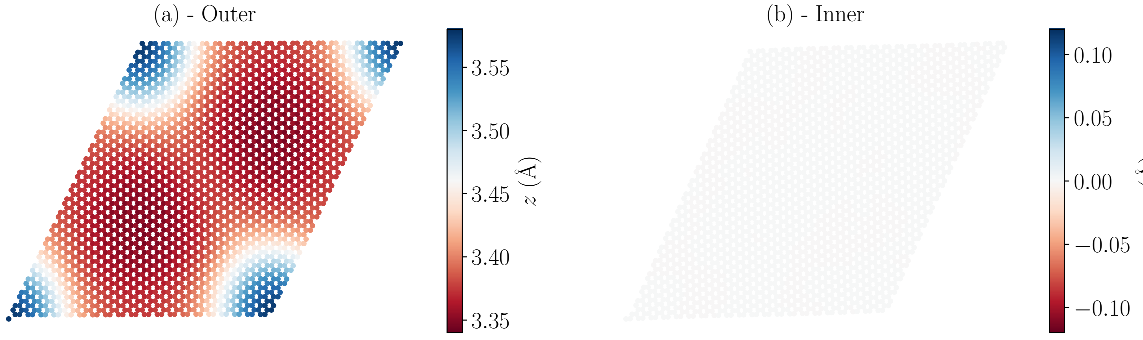


**Supplementary Figure** 1. **Out-of-plane corrugation effects of TTG at 1.61°.** **(a)** Outer layer above the middle, twisted layer. The lower layer essentially has an identical relaxation pattern. **(b)** Inner, twisted layer. The inner layer is taken as the origin of the $z$-axis.

*Density Functional Theory* In Fig. 2, we show the band structures of TTG at 3.15° and 2.45° from DFT. The low-energy electronic structure consists of a set of flat bands which intersect a Dirac cone with a large Fermi velocity. Overall, we find good agreement between the DFT electronic structure and the atomistic tight binding model, which shall be described in the next section. The main difference between the methods is where the flat bands intersect the Dirac cone. In the DFT calculations, the flat bands intersect the Dirac cone at lower energies than the Dirac point, but in the tight binding calculations they intersect at higher energies than the Dirac point. To improve the model's accordance with both our DFT simulations and the ones from Ref. 2, we include an additional onsite potential energy that only acts on the middle layer of the system −35 meV.


* Corresponding author: dante.kennes@rwth-aachen.de
† Corresponding author: klebl@physik.rwth-aachen.de

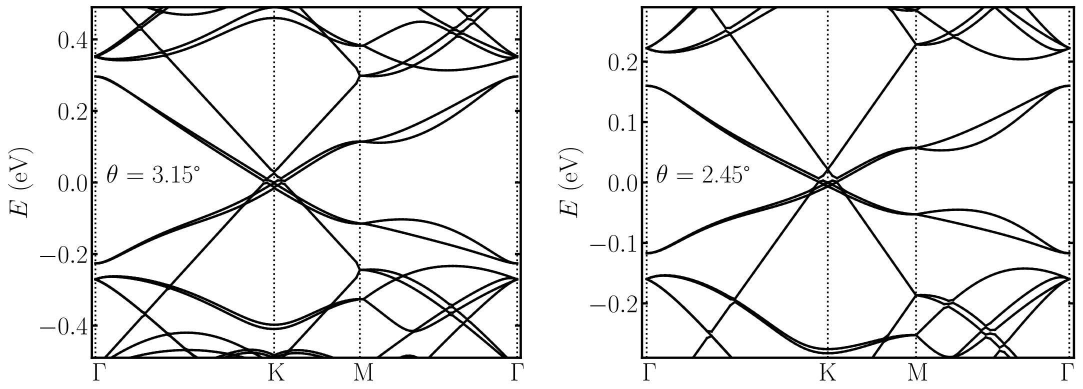


**Supplementary Figure 2. DFT band structure along the high symmetry path of the moiré Brillouin zone.**

*Atomistic Hartree Theory* The method outlined here follows that of Ref. 3. Also see Ref. 4 for a similar method, or Refs. 5, 6 for continuum model approach, or Ref. 7 for a orbital approach.

The long-ranged electron interaction contribution to the Hamiltonian can be included through

$$H^H_{ii} = \int \mathrm{d}\boldsymbol{r}\, \phi_z^2(\boldsymbol{r} - \boldsymbol{\tau}_i) V_{\mathrm{H}}(\boldsymbol{r}), \tag{1}$$

where $\phi_z(\boldsymbol{r})$ is the $\mathrm{p}_z$ orbitals of the carbon atoms and $V_{\mathrm{H}}(\boldsymbol{r})$ is the Hartree potential of these orbitals. The Hartree potential is calculated from the convolution of the electron density $n(\boldsymbol{r})$ and the screened interaction $W(\boldsymbol{r})$, given by

$$V_{\mathrm{H}}(\boldsymbol{r}) = \int \mathrm{d}\boldsymbol{r}'\, W(\boldsymbol{r} - \boldsymbol{r}')[n(\boldsymbol{r}') - n_0(\boldsymbol{r}')], \tag{2}$$

where $n_0(\boldsymbol{r})$ is a reference electron density of the uniform system. The electron density is determined through

$$n(\boldsymbol{r}) = \sum_{n\boldsymbol{k}} f_{n\boldsymbol{k}} |\psi_{n\boldsymbol{k}}(\boldsymbol{r})|^2 \tag{3}$$

where $\psi_{n\boldsymbol{k}}(\boldsymbol{r})$ is the Bloch eigenstate of the tight binding model, with subscripts $n$ and $\boldsymbol{k}$ denoting the band index and crystal momentum, respectively; $N_{\mathrm{k}}$ is the number of k-points in the summation of the electron density, and $f_{n\boldsymbol{k}} = 2\Theta(\varepsilon_{\mathrm{F}} - \varepsilon_{n\boldsymbol{k}})$ is the spin-degenerate occupancy of state $n\boldsymbol{k}$ (where $\varepsilon_{\mathrm{F}}$ is the Fermi energy and $\varepsilon_{n\boldsymbol{k}}$ is the eigenvalue of that state). Inserting the Bloch states in Eq. (3) gives

$$n(\boldsymbol{r}) = \sum_j n_j \chi_j(\boldsymbol{r}), \tag{4}$$

where $\chi_j(\boldsymbol{r}) = \sum_{\boldsymbol{R}} \phi_z^2(\boldsymbol{r} - \boldsymbol{\tau}_j - \boldsymbol{R})$ (with $\boldsymbol{R}$ denoting the moiré lattice vectors) and the total number of electrons on the $j$-th $\mathrm{p}_z$-orbital in the unit cell being determined by $n_j = \sum_{n\boldsymbol{k}} f_{n\boldsymbol{k}} |c_{n\boldsymbol{k}j}|^2 / N_{\mathrm{k}}$, with $c_{n\boldsymbol{k}j}$ denoting the coefficients of the eigenvectors of the tight binding model.

The reference density is taken to be that of a uniform system, $n_0(\boldsymbol{r}) = \bar{n} \sum_j \chi_j(\boldsymbol{r})$, where $\bar{n}$ is the average of $n_j$ over all atoms in the unit cell, which is related to the filling per moiré unit cell $\nu$ through $\bar{n} = 1 + \nu/N$, where $N$ is the total number of atoms in a moiré unit cell [4]. This reference density is taken to prevent overcounting the intrinsic graphene Hartree contribution which should be included in the hopping parameters.

In our atomistic model, we neglect contributions to the electron density from overlapping $\mathrm{p}_z$-orbitals that do not belong to the same carbon atom, which is equivalent to treating $\phi_z^2(\boldsymbol{r})$ as a delta-function. Therefore, we calculate the Hartree on-site energies using

$$H^H_{ii} = \sum_{j\boldsymbol{R}} (n_j - \bar{n}) W_{\boldsymbol{R}ij}, \tag{5}$$

where $W_{\boldsymbol{R}ij} = V_0 / |(\boldsymbol{R} + \boldsymbol{\tau}_j - \boldsymbol{\tau}_i)|$, where $V_0$ is the Coulomb potential energy scale with a dielectric constant of 1. If $\boldsymbol{R} = 0$ and $i = j$, we set $W_{0,ii} = 17$ eV [8].

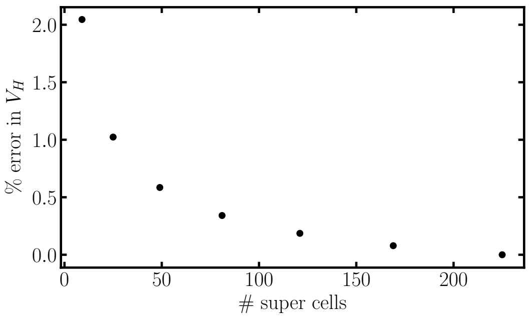


**Supplementary Figure 3. Convergence of the self-consistent Hartree calculations at a twist angle of 1.6°**. The doping level is set to $\nu = +3$ electrons and the self-consistent calculation is based off the charge density which comes out of the non-interacting tight-binding model. The relative error to the converged value is shown as a function of number of supercells. We assume $15 \times 15 = 225$ supercells to be sufficient for a converged result as the slope of the line has almost decayed to zero.

To obtain a self-consistent solution of the equations, we use a $8 \times 8$ $\boldsymbol{k}$-point grid to sample the first Brillouin zone to converge the electron density, and we sum over a $11 \times 11$ supercell of moiré unit cells to converge the onsite energy. Linear mixing of the electron density is performed with a mixing parameter of 0.1 or less. Typically, the Hartree potential converges to an accuracy of better than 0.1 meV per atom within 100 iterations (see Fig. 3).

As mentioned in the main text, we find strong similarities between the effect of Hartree interactions in TTG and TBG [3–7]. This is perhaps not surprising as TTG can be mapped onto a system that is TBG (at a different twist angle) and a graphene layer [9], such that we might expect similar behaviour from the constitutive parts. We find the flat bands are quite sensitive to the Hartree interactions, while the Dirac cone with large Fermi velocity is completely insensitive to these interactions. Upon electron doping (as seen in the main text and later on), the flat band electronic structure strongly distorts, with the states at the edge of the Brillouin zone increasing in energy relative to the states at the centre. The converse is true for hole doping.

These strong band deformations arise because of the strongly peaked local density of states (LDOS) in the AAA regions, with the strongest weights in the inner, twisted layer. Upon removing (adding) electrons, they are practically only taken from (added to) the AAA regions. This localisation of the flat band LDOS gives rise to a strongly varying Hartree potential, as was also found in TBG [3–7]. In Fig. 4 **(c,d)** we show that the Hartree potential is strongly peaked in the AAA regions when 3 electrons are removed from 1.61° TTG. This Hartree potential substantially varies with doping level but does not change significantly with twist angle, as summarised in Fig. 4 **(a,b)**.

In Fig. 4 **(a)** we plot how the layer-dependent constant contribution to the Hartree potential ($\Delta_l$) changes with doping level for several twist angles. Interestingly, we find that the outer layers (1/3) have a zero constant contribution ($\Delta_{1/3} = 0$) for all doping levels and twist angles. However, the central layer (2) has a constant contribution which changes significantly with doping level, but hardly changes with twist angle. When doping within the flat bands, we find that the constant contribution increases when electrons are added, but it becomes more negative when electrons are removed. This occurs because of electrons mainly being added/removed from the central layer. The change in this constant contribution is approximately linear ($\Delta_2 \approx \Delta_2' \nu$) when doping inside of the flat bands. Doping the system outside of the flat bands causes the magnitude of the constant contribution to decrease, which reflects the fact that electrons are now being removed/added from the outer layers where the Dirac cone with large Fermi velocity resides.

In Fig. 4 **(b)** we plot the scale of the cosine contribution to the Hartree potential, as calculated by

$$V_l(\nu) = \frac{\sum_i V_H(\nu, \boldsymbol{\tau}_{il}) \cdot v_c(\boldsymbol{\tau}_{il})}{\sum_j v_c(\boldsymbol{\tau}_{jl}) \cdot v_c(\boldsymbol{\tau}_{jl})}, \tag{6}$$

where

$$v_c(\boldsymbol{\tau}_{il}) = \sum_j \cos(\boldsymbol{b}_j \cdot \boldsymbol{\tau}_{il}). \tag{7}$$

Here $\boldsymbol{b}_j$ is the three shortest reciprocal moiré lattice vectors [3] and note the summations only run over the atoms in layer $l$. The scale of the cosine contribution to the Hartree potential is largest in the inner layer (2), as this is where electrons are mainly being added/removed from. Doping the TTG inside of the flat bands causes an approximately linear change on the cosine contribution to the Hartree potential ($V_l \approx V_l' \nu$), which is similar to TBG [3–7]. Upon doping outside of the flat bands, the cosine contribution stops changing significantly as electrons are no longer being added/removed from the peaked LDOS AAA regions.

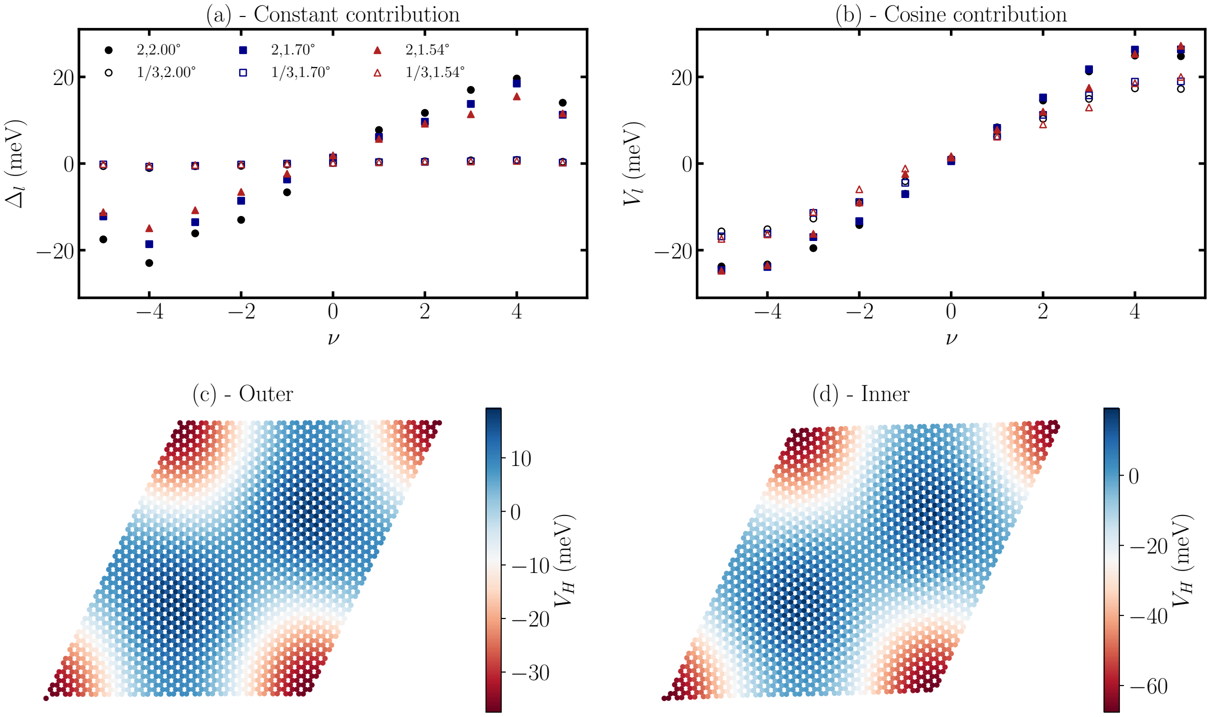


**Supplementary Figure** 4. **Hartree potential dependence on twist angle and doping level for the inner and outer layers.** **(a)** Constant contribution to the Hartree potential on each layer as a function of doping level for a number of twist angles. Legend shows the layer (1/3 or 2) and the twist angle convention used for the symbols. **(b)** Cosine contribution to the Hartree potential on each layer as a function of doping level for a number of twist angles. **(c)** Hartree potential on the outer layers for 1.61° at $\nu = -3$. **(d)** Hartree potential on the inner layer for 1.61° at $\nu = -3$.

In Fig. 5, the dependence of the Hartree potential on doping and dielectric environment of a 2° structure is shown. As seen in Fig. 5 **(a)**, for the larger dielectric constant of 4, which models the hexagonal boron nitride (hBN) substrate, the constant contribution to the Hartree potential reduces on the middle layer by 65%. Whereas, as seen in Fig. 5 **(b)**, the cosine contribution is significantly more robust with respect to the dielectric environment, where a maximum of a 30% reduction in the Hartree potential is observed. This insensitivity of the Hartree potential to the dielectric environment was also found in tBLG [3], where it was suggested to occur because of the already large internal dielectric constant of tBLG.

The above Hartree potential can be well parameterised by the following equation

$$H^H_{iil} \approx \Delta'_l \nu + V'_l \nu \sum_j \cos(\boldsymbol{b}_j \cdot \boldsymbol{\tau}_{il}), \tag{8}$$

where $\Delta'_l$ is the constant contribution on layer $l$, $V'_l$ is the scale of the Hartree potential on layer $l$, $\nu$ is the doping level, $\boldsymbol{b}_j$ are the three shortest reciprocal lattice vectors, and $\boldsymbol{\tau}_{il}$ are the atomic positions of carbon atom $i$ in layer $l$. A similar form was used to parameterise the Hartree potential of TBG [3]. Note that the AAA regions have to reside at the corners of the moiré unit cell for this equation to work - otherwise one must rigidly shift the potential such that the peaks of the potential occur in the AAA region. This allows one to efficiently investigate other doping levels and twist angles that are not calculated self-consistently, as the Hartree potential varies smoothly in $\nu$-space and does not change significantly in $\theta$-space close to the magic angle. Note that these Hartree theory calculations were not performed with the intrinsic symmetric polarisation potential.

In the RPA calculations described later, we take $\Delta'_2 = 5$ meV, $V'_{1/3} = 4$ meV and $V'_2 = 6$ meV. These values are based off the dielectric environment of air, but as we have shown in Fig. 5, there is little change to the cosine contribution parameters when taking into account the dielectric environment of hBN. The constant contribution is more sensitive to the dielectric environment. As the constant contribution only shifts the flat bands, but the cosine contribution causes significant deformations, the cosine parameters are the more important contribution. Therefore, the employed parameters should still provide reliable comparisons against experiments. In Ref. 10 a similar approach

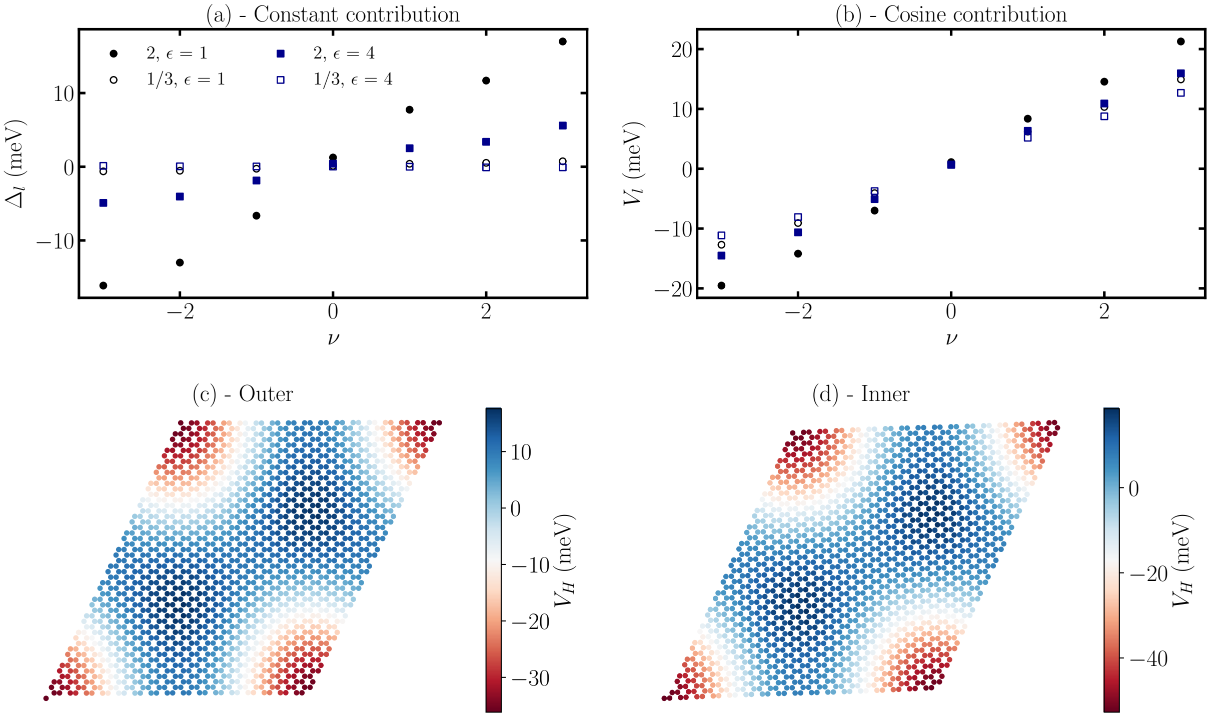


**Supplementary Figure** 5. **Hartree potential dependence on doping level and dielectric constant for the inner and outer layers.** All figures are for a twist angle of 2°. **(a)** Constant contribution to the Hartree potential on each layer as a function of doping level for several dielectric constants, where the legend shows the layer (1/3 or 2) and the dielectric constant (1 or 4) convention used for the symbols. **(b)** Cosine contribution to the Hartree potential on each layer as a function of doping level for a number of twist angles. **(c)** Hartree potential on the outer layers for 2° at $\nu = -3$ with dielectric constant of 4. **(d)** Hartree potential on the inner layer for 2° at $\nu = -3$ with dielectric constant of 4.

was taken for TBG and excellent agreement was found with experiments, which suggests that it should work for TTG too.

*Electric Field* We include an electric field through

$$H^E_{iil} = \pm\Delta_D, \tag{9}$$

where $\Delta_D$ is the additional potential that electrons feel on the outer layers of TTG, the sign of which depends on the layer and direction of the field.

We performed self-consistent Hartree calculations with $\Delta_D = 10$ meV to investigate the effect of screening from TTG has on the perpendicular electric field. We found that at this electric field strength, the intrinsic Hartree potential is not significantly effected other than an additional layer-dependent onsite potential which screens the perpendicular electric field. Therefore, we can use the Hartree potential in the absence of a field, and screen the field by a constant.

To extract an effective dielectric constant which screens a perpendicular field, we calculate the following $\epsilon_r = 2\Delta_D/(\Delta_1 - \Delta_3 + 2\Delta_D)$, where $\Delta_{1/3}$ are the layer-dependent onsite Hartree potentials. For a twist angle of 2° and doping level of $\nu = 3$ we find a dielectric constant of $\epsilon_r = 3.35$, and at charge neutrality we find $\epsilon_r = 1.87$. Overall, we find TTG has a dielectric constant of approximately 2-3 for screening perpendicular electric fields. This value of the perpendicular effective dielectric constant is not far from the value of 3-4 for a trilayer graphene system obtain from DFT calculations of Ref. 11.

With a dielectric constant of 3 and an onsite potential energy of $\Delta_D = \pm 30$ meV, the corresponding displacement field is approximately 0.25 Vnm$^{-1}$. In the experiments of Ref. 12, the optimal electric field corresponds to a 0.5 Vnm$^{-1}$ displacement field. This is within a factor of 2 of our calculations, which is reasonable agreement.

*Full Atomistic Hamiltonian* As discussed in the Methods section of the main text, the full tight binding Hamiltonian consists of the following contributions:

$$\hat{H} = \hat{H}^0 + \hat{H}^H + \hat{H}^\Delta + \hat{H}^E, \quad \mathsf{H} = \sum_{ij\sigma} H_{ij} c^\dagger_{i\sigma} c_{j\sigma}, \tag{10}$$

In Fig. 6 we display some additional band structure figures to that shown in the main text for different twist angles. Specifically, we show a calculation with a self-consistent Hartree potential and an intrinsic-symmetric polarisation potential, but without an electric field. We can clearly see that the Hartree potential causes significant band distortions for all twist angles, with the relative distortions at smaller twist angles being more pronounced.

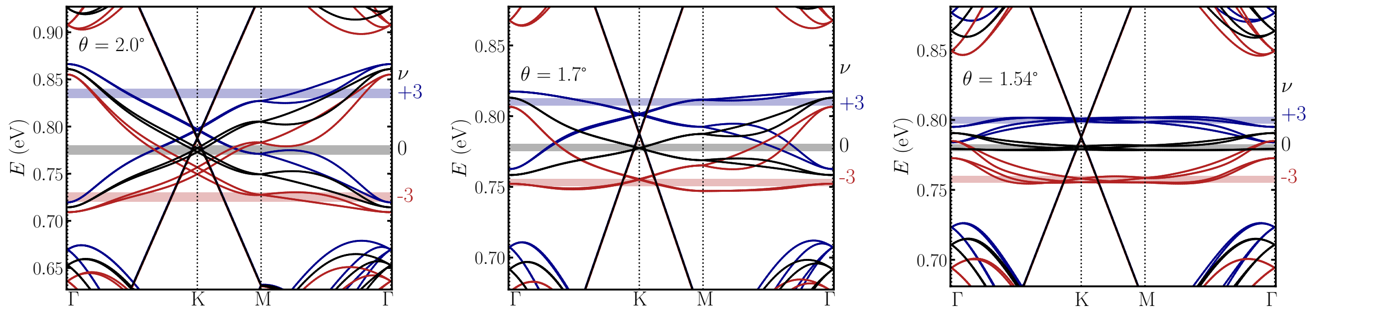


**Supplementary Figure** 6. **Band structure along high symmetry path for several twist angles and doping levels, but without an applied electric field.**

We show the Fermi contour of MATTG in Fig. 7 for a set of three fractional fillings of the moiré bands: $\nu \in \{-2.3, -2.5, -2.7\}$. Nesting is only supported at a vector $\boldsymbol{q}$ close to Γ that is incommensurate with the Brillouin zone. Thus, magnetic ordering at $\boldsymbol{q} \neq 0$ is unlikely to occur. As expected from the symmetry analysis presented in the manuscript, the Fermi surface possesses a six-fold rotational symmetry. Contrary to TBG, twisted trilayer graphene is not two-fold symmetric $C_{2x(y)}$ around the axis $x(y)$ lying within the middle graphene sheet, but only exhibits the mirror reflection symmetry $\sigma_h$. Hence, the symmetry of Fermi surface is reduced with respect to TBG.

*Magnetic RPA* To study magnetism, we add a Hubbard interaction acting on the graphene $p_z$ orbitals in the Hamiltonian $\mathsf{H}$:

$$\mathsf{H}^{\mathrm{U}} = \mathsf{H} + \mathsf{H}^{\mathrm{I}}, \quad \mathsf{H}^{\mathrm{I}} = \sum_{i\sigma} U\, n_{i,\sigma} n_{i,\bar{\sigma}}. \tag{11}$$

We employ the well established method of static, long-wavelength magnetic random phase approximation to treat the four-fermion term $\mathsf{H}_{\mathrm{I}}$ as presented in Ref. 13. To analyze magnetic ordering tendencies, we calculate the magnetic susceptibility $\hat{\chi}_0$:

$$\hat{\chi}_0 = \hat{\chi}_0(\boldsymbol{q} = q_0 = 0) = \frac{T}{N_{\boldsymbol{k}}} \sum_{\boldsymbol{k},k_0} \hat{G}(\boldsymbol{k}, k_0) \circ \hat{G}(\boldsymbol{k}, k_0)^{\mathrm{T}}. \tag{12}$$

The Green's function $\hat{G}(\boldsymbol{k}, k_0) = G_{ij}(\boldsymbol{k}, k_0)$ as a function of Matsubara frequency $k_0$, moiré momentum $\boldsymbol{k}$ is given by

$$\hat{G}(\boldsymbol{k}, k_0) = (ik_0\mathbb{1} - \hat{H}(\boldsymbol{k}) + \mu\mathbb{1})^{-1}, \tag{13}$$

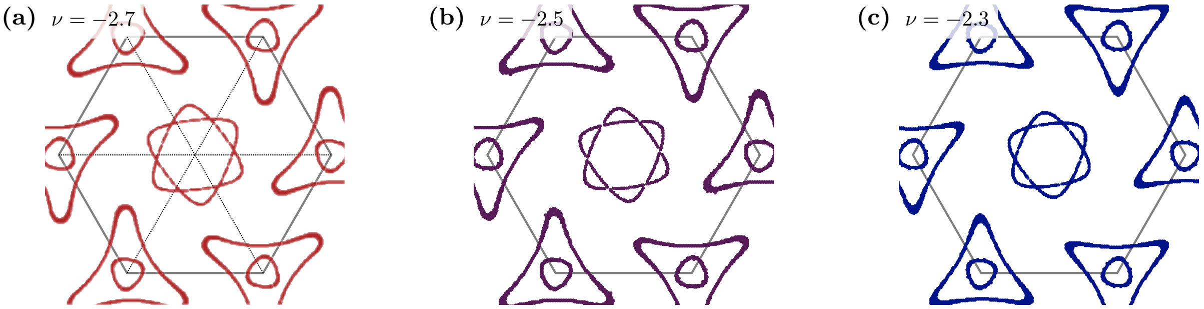


**Supplementary Figure** 7. **Fermi contours for three fractional fillings of the moiré bands.** At the fillings shown in **(a),(b),(c)**, magnetic ordering at $\boldsymbol{q} \neq 0$ is unlikely due to the approximate nesting vector being incommensurate with the Brillouin zone. The Fermi surface is six-fold rotational symmetric with respect to the Γ point of the Brillouin zone as expected from the symmetry analysis presented in the manuscript.

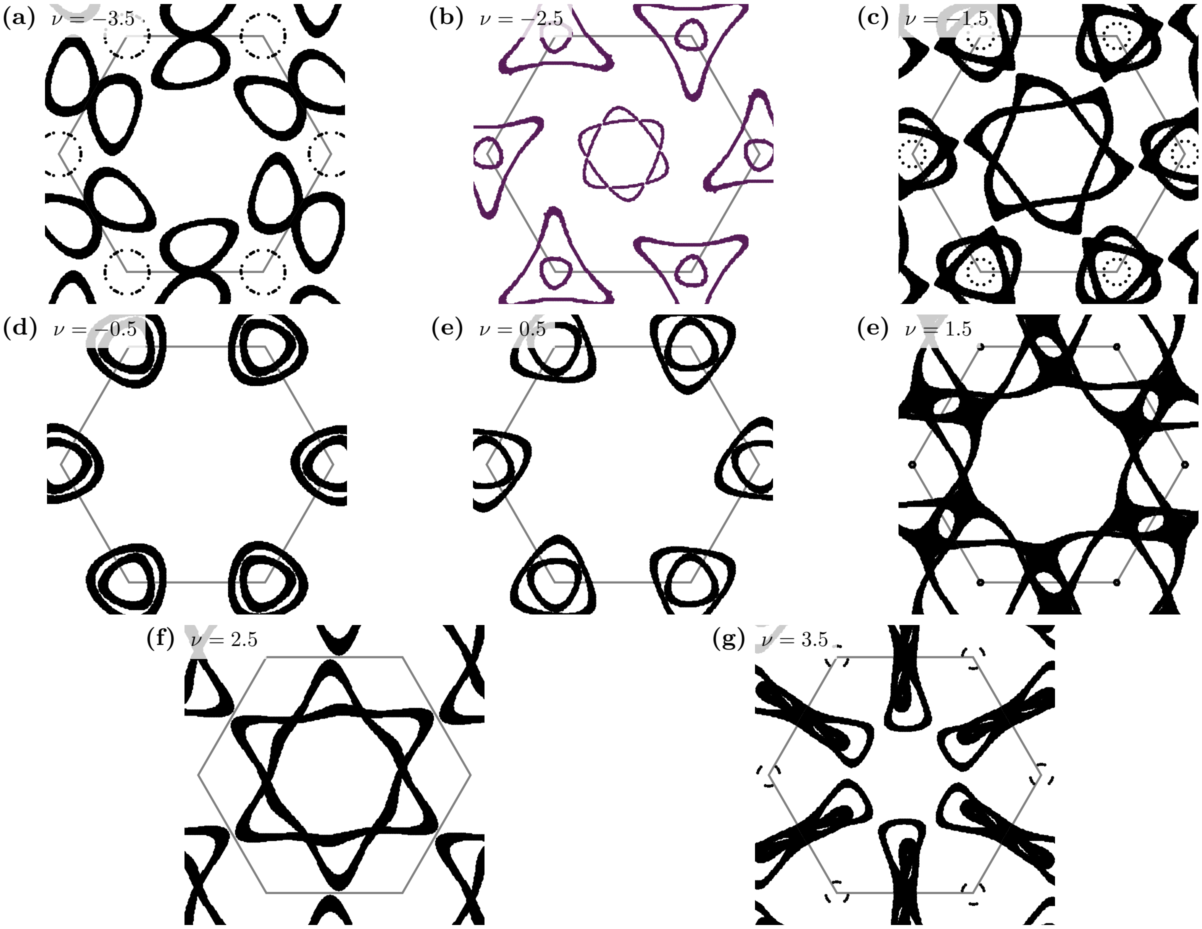


**Supplementary Figure** 8. **Fermi contours for half-integer filling values of the moiré flat bands. (a-g)** Filling range in integer steps from $\nu = -3.5$ to $\nu = +3.5$.

with $H(\boldsymbol{k})$ the "non-interacting" tight-binding Hamiltonian *including* the Hartree corrections and $\mu$ the chemical potential corresponding to the filling factor used in the Hartree potential.

From the extended Stoner criterion [14], we find that the critical Hubbard-$U$ needed for the onset of magnetic ordering is given by $U_{\mathrm{c}} = -1/\lambda_0$, with $\lambda_0$ the lowest eigenvalue of $\hat{\chi}_0$. The magnetic ordering is proportional to the corresponding eigenvector $\vec{v}_0$. For numerical evaluation of the Matsubara sum in Eq. (12), we use the exact same frequency grid presented in Ref. 10 and thus are able to take into account the effect of low-temperature instabilities consistently by using the temperature-dependent number of frequencies presented in Table I. We sample the moiré Brillouin zone with $N_{\boldsymbol{k}} = 24$ points for the RPA simulations. To show that this resolution in $N_{\boldsymbol{k}}$ is sufficient, we performed a convergence analysis at the exemplary filling of $\nu = -2.5$ and temperature $T = 1.32\,\mathrm{K}$ (see Fig. 9).

**Supplementary Table** I. Inverse temperatures, temperatures and number of Matsubara frequencies in the RPA summations used for the simulation of the superconducting dome. The spacing of $\beta$ (and $T$) is chosen to be logarithmic. The parameters $T = 1.32\,\mathrm{K}$ and $N_\omega = 500$ were used for Figs. 1 **(c)** and **(d)** of the main text.

| $\beta\,(\mathrm{eV}^{-1})$ | 50000 | 32374 | 20961 | 13572 | 8788 | 5690 | 3684 | 2385 | 1544 | 1000 |
|---|---|---|---|---|---|---|---|---|---|---|
| $T$ (K) | 0.23 | 0.36 | 0.55 | 0.86 | 1.32 | 2.04 | 3.15 | 4.87 | 7.52 | 11.6 |
| $N_\omega$ | 1200 | 966 | 780 | 620 | 500 | 500 | 500 | 500 | 500 | 500 |

The three types of magnetic ordering are shown in Fig. 10. In Figure 1 **(d,e,f)** of the main text, we do not differentiate between the two types of antiferromagnetic ordering [Fig. 10 **(a,b)**] as the consequences for superconductivity are very similar. For nonzero electric displacement field, i.e. $\Delta_D = \pm 30\,\mathrm{meV}$, the types of ordering do not differ

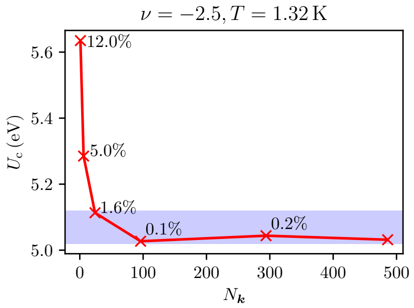


**Supplementary Figure** 9. **Convergence of the magnetic susceptibility.** The critical interaction strength $U_c$ is shown as a function of number of sampling points $N_{\boldsymbol{k}}$ in the Brillouin zone for $\nu = -2.5$ and $T = 1.32\,\mathrm{K}$. The region shaded in blue indicates what results we accept as converged. The relative error of $U_c$ to the value at $N_{\boldsymbol{k}} = 486$ is annotated. Note that the type of ordering is the same AFM ordering for all BZ samplings.

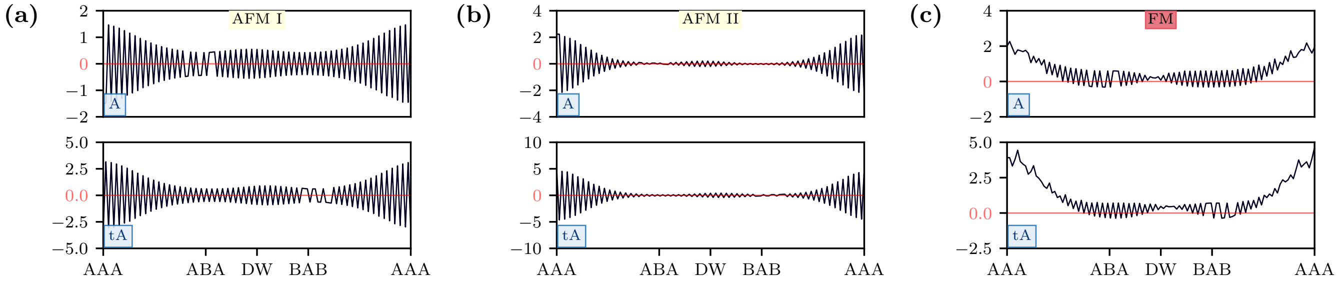


**Supplementary Figure** 10. **Magnetic orderings found for MATTG.** Linecuts of the leading magnetic order parameter along the diagonal of the rhombus shaped unit cell. Only two layers are shown as the bottom layer contribution of the order parameter is equivalent to the top layer contribution for all ordering shown. Panel **(a)** shows the first type of antiferromagnetic (AFM) order that is a carbon-scale AFM order modulated in each layer and on the moiré scale. Panel **(b)** shows AFM order on the carbon scale stronger modulation on the moiré scale such that it exhibits a node in the top layer ABA/BAB regions. Panel **(c)** shows ferromagnetic (FM) order with some reminiscent ferrimagnetism in the ABA/BAB regions. In every case, the middle layer (panel titled "tA") has a much larger amplitude than the outer layers ("A").

qualitatively, despite the breaking of $C_{2z}$ symmetry. Fig. 10 shows that the weight of the magnetic instabilities is mainly in the middle layer in the AAA regions, which is a manifestation of the weight of the electronic wavefunctions mostly being centered around these points (see Fig. 1 **(c)** of the main text). For the $\nu - T$ region where we determine the superconducting gap (Fig. 1 **(d)** of the main text), Fig. 11 shows $U_c$ **(a)** and the type of magnetic order **(b)** using the order parameter

$$\zeta = \frac{1}{\sqrt{N}} \left| \sum_i v_0^i \right| , \tag{14}$$

where $N$ is the number of carbon atoms per unit cell.

*Pairing Vertex in fluctuation-exchange approximation (FLEX)* To account for pairing instabilities mediated by charge- and spin-fluctuation exchange, we derive a microscopic pairing interaction $\hat{\Gamma}_2$ in the fluctuation-exchange approximation (FLEX) that incorporates effects of transverse and longitudinal spin-fluctuations, see Fig. 13. In terms of the full atomistic RPA susceptibility $\chi_0$, the scattering between spin-singlet Cooper pairs is described by the pairing vertex [15]

$$\hat{\Gamma}_2(q) = U\mathbb{1} - \frac{U^2 \hat{\chi}_0(q)}{\mathbb{1} + U\hat{\chi}_0(q)} + \frac{U^3 \hat{\chi}_0^2(q)}{\mathbb{1} - U^2 \hat{\chi}_0^2(q)} . \tag{15}$$

In the static, long-wavelength limit ($q \to 0$), we hence fall back to the computation of the atomistic susceptibility matrix, see paragraph 'Magnetic RPA'. The real-space dependence of the interaction vertex $\hat{\Gamma}_2 = \Gamma_{2,ij}$ is shown in Fig. 14. Fixing one of the two real-space indices to either the AAA, ABA or DW regions, the interaction profile throughout the unit cell strongly depends on the spin-fluctuation spectrum predicted by the RPA analysis. For filling ranges dominated by AFM fluctuations, the interaction vertex is staggered throughout the moiré unit cell of

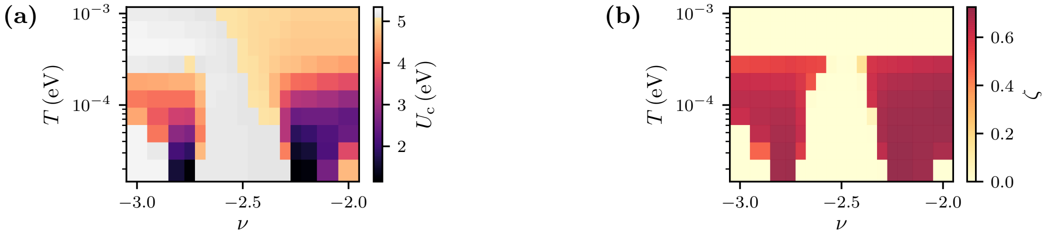


**Supplementary Figure** 11. **Magnetic instabilities of MATTG between filling factors $\nu = -2, -3$.** The left panel **(a)** emphasizes the regions where superconducting order by a spin fluctuation mechanism is possible by graying out the regions where $U_c \geq U = 5.11\,\mathrm{eV}$. On the right hand side **(b)**, we plot the magnetic order parameter $\zeta$ that smoothly interpolates between AFM ($\zeta = 0$) and FM ($\zeta = 1$) order.

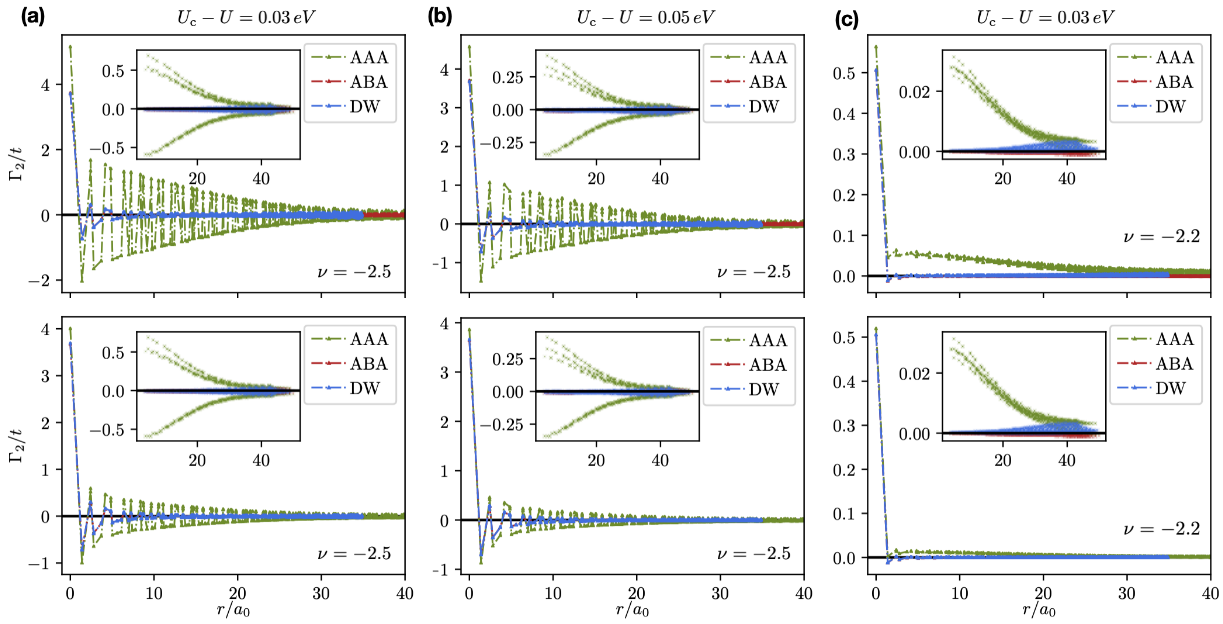


**Supplementary Figure** 12. **Real-space profile of the effective pairing vertex $\hat{\Gamma}_2$ in the middle (upper panels) and outer layers (lower panels) of MATTG. (a,b)** Close to an antiferromagnetic (AFM) instability, the pairing vertex is staggered in real-space: Strong on-site repulsion inherited from the repulsive Hubbard-$U$ is followed by nearest-neighbor attraction. Real-space profiles are shown starting from an atom located in the AAA, ABA or DW region of MATTG, respectively. The inset shows the interlayer component, which happens to be an order of magnitude smaller than comparable intralayer terms. The overall amplitude of the interaction is enhanced in the vicinity of the magnetic phase: As $U \to U_c$ the amplitude of the pairing interaction increases notably in the AAA regions of the middle layer as depicted in sub panels **(a)** and **(b)**. The amplitude in the outer layer is merely affected. **(c)** Close to a ferromagnetic (FM) magnetic instability at, the spin-fluctuation mediated pairing vertex is purely repulsive throughout the moiré unit cell.

MATTG: While strong on-site repulsion is inherited from the initial Hubbard-$U$ term, AFM spin-fluctuation exchange generates *attractive* terms living on the nearst-neighbor bonds in the single graphene sheets. In contrast, the effective spin-singlet interaction is mostly repulsive in the vicinity of FM ordering tendencies.

We stress that the interlayer component of the interaction is an order of magnitude smaller than comparable interlayer terms. This leads to the conclusion, that on the atomistic scale, in-plane Cooper pairs are strongly favoured by spin-fluctuation exchange. These observations are not surprising as the interlayer coupling between the single graphene sheets in the non-interacting Hamiltonian is supressed by the same amount as expected for van der Waals heterostructures as MATTG.

The overall amplitude of the effective pairing vertex $\hat{\Gamma}_2$ increases in the vicinity of the magnetic instability, i.e. if $U \to U_c$. As the system shows an increased susceptibility for magnetic fluctuations in the middle layer of MATTG (especially in the AAA regions), the divergence of the interaction is first observed there. To calculate a meaningful $\nu - T$ phase diagram at fixed Hubbard interaction $U$ as shown in the manuscript, we hence circumvent the divergence

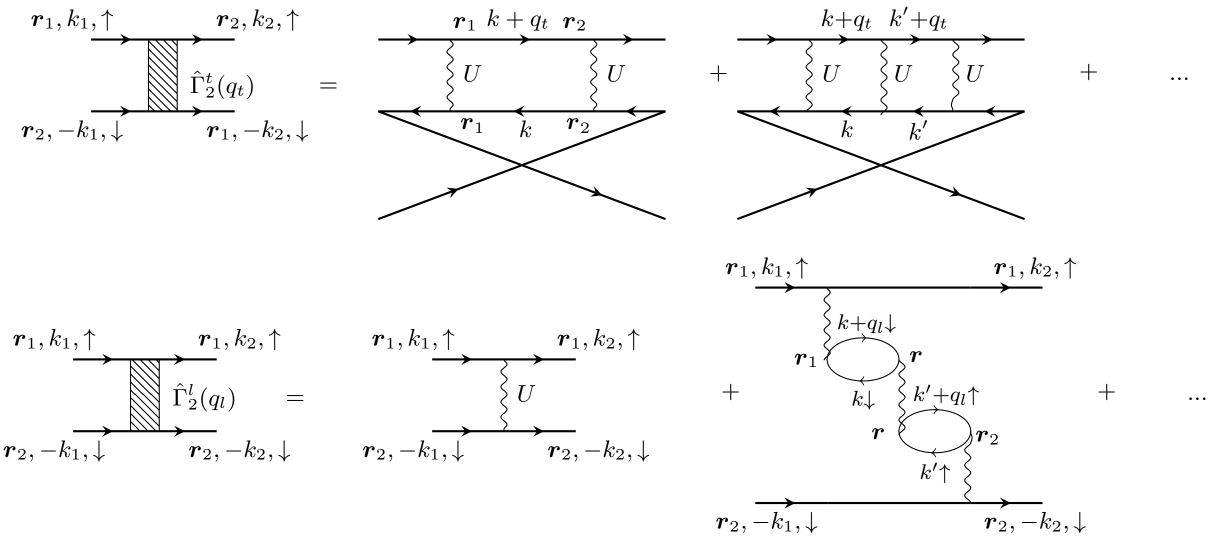


**Supplementary Figure** 13. **Diagrams contributing to the transverse/longitudinal spin-fluctuation mediated pairing interaction $\hat{\Gamma}_2(q)$ in the spin-singlet channel. Upper Row:** Transverse Spin-fluctuations $\hat{\Gamma}_2^t(q_t)$. The momentum transfer occurring in the polarization function in RPA is given by $q_t = k_1 + k_2$ due to momentum conservation. **Lower Row**: Longitudinal Spin-Flututaions $\hat{\Gamma}_2^l(q_l)$. The momentum transfer occurring in the polarization function in RPA is given by $q_l = k_1 - k_2$. Only an even number of particle-hole bubbles is allowed in the diagrammatic expansion in order to preserve the spin in the upper and lower leg of the pairing interaction. The diagrams that are resummed in the longitudinal channel are connected to the particle-hole susceptibility describing screening effects of the bare Coulomb interaction.

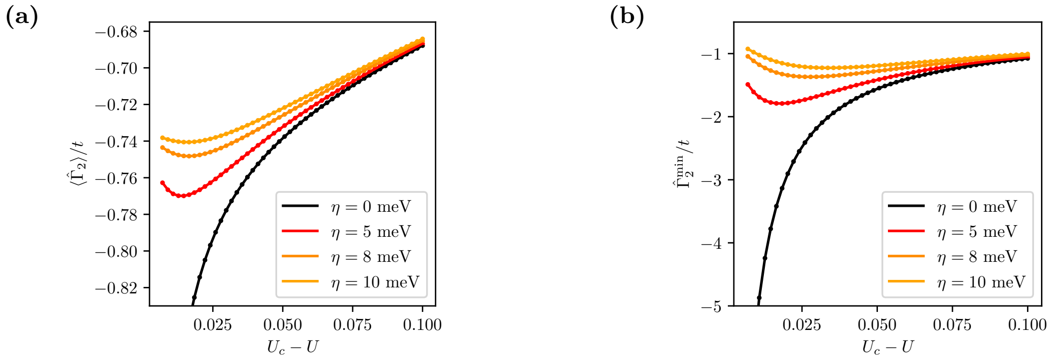


**Supplementary Figure** 14. **Pairing vertex as a function of broadening**. Average **(a)** and minimum **(b)** value of the attractive interaction on nearest-neighbor bonds originating from the effective spin-mediated pairing vertex $\hat{\Gamma}_2$ as function of Hubbard-$U$ for different choices of the broadening parameter $\eta$.

for values $U \lesssim U_c$ at certain fillings by applying a Lorentzian broadening to the interaction vertex

$$\hat{\Gamma}_2^{\eta}(q) = \mathrm{Re}\left[U\mathbb{1} - \frac{U^2\hat{\chi}_0(q)}{\mathbb{1} + U\hat{\chi}_0(q) + i\eta\mathbb{1}} + \frac{U^3\hat{\chi}_0^2(q)}{\mathbb{1} - U^2\hat{\chi}_0^2(q) + i\eta\mathbb{1}}\right] \tag{16}$$

In all calculations leading to the phase diagram in Fig. 1 **(d)** in the manuscript, we set the broadening parameter to $\eta = 8\,\mathrm{meV}$. This effectively avoids a divergence of the interactions in the AAA regions in the middle layer. We checked that different choices of the broadening parameter $\eta$ do not change our results qualitatively. An analysis of the pairing vertex $\hat{\Gamma}_2^{\eta}$ as a function of broadening $\eta$ and Hubbard-$U$ is shown in Fig. 14.

*Bogoliubov de-Gennes equations* To analyze the superconducting properties of the system, we decouple the effective pairing vertex $\hat{\Gamma}_2$ in mean-field approximation, allowing only for symmetric spin-singlet bond order parameters $\Delta_{ij} = \Delta_{ji}$ due to the proximity to AFM tendencies in between the integer fillings

$$\hat{\Delta}(\boldsymbol{k}) = \Delta_{nm}(\boldsymbol{k}) = -\frac{1}{2N}\sum_{\boldsymbol{k}'\sigma}\Gamma_{2,nm}(\boldsymbol{q} = \boldsymbol{k} - \boldsymbol{k}', q_0 = 0) \times \sigma\langle c_{n\sigma}(\boldsymbol{k}')c_{m\bar{\sigma}}(-\boldsymbol{k}')\rangle_{\mathrm{MF}}, \tag{17}$$

The resulting mean-field Hamiltonian can be rewritten in the $2N$-dimensional Nambu spinor basis $\psi^\dagger_{\boldsymbol{k}} = (\vec{c}_{\boldsymbol{k}\uparrow} \ \vec{c}^{\,\dagger}_{-\boldsymbol{k}\downarrow})^{\mathrm{T}}$

$$\mathsf{H}_{\mathrm{MF}} = \sum_{\boldsymbol{k}} \psi^\dagger_{\boldsymbol{k}} \begin{pmatrix} \hat{H}(\boldsymbol{k}) & \hat{\Delta}(\boldsymbol{k}) \\ \hat{\Delta}^\dagger(\boldsymbol{k}) & -\hat{H}(-\boldsymbol{k}) \end{pmatrix} \psi_{\boldsymbol{k}} + \mathrm{const.} \tag{18}$$

This Bogoliubov de-Gennes (BdG) bilinear form is diagonalized by a block-structured unitary transform $\hat{U}_{\boldsymbol{k}}$

$$\begin{aligned} H_{\mathrm{MF}} &= \sum_{\boldsymbol{k}} \psi^\dagger_{\boldsymbol{k}} \begin{pmatrix} \hat{H}(\boldsymbol{k}) & \hat{\Delta}(\boldsymbol{k}) \\ \hat{\Delta}^\dagger(\boldsymbol{k}) & -\hat{H}(-\boldsymbol{k}) \end{pmatrix} \psi_{\boldsymbol{k}} = \sum_{\boldsymbol{k}} \left(\hat{U}_{\boldsymbol{k}}\psi_{\boldsymbol{k}}\right)^\dagger \begin{pmatrix} \hat{E}_{\boldsymbol{k}} & 0 \\ 0 & -\hat{E}_{\boldsymbol{k}} \end{pmatrix} \left(\hat{U}_{\boldsymbol{k}}\psi_{\boldsymbol{k}}\right) \\ \hat{U}_{\boldsymbol{k}} &= \begin{pmatrix} \hat{u}_{\boldsymbol{k}} & -\hat{v}_{\boldsymbol{k}} \\ \hat{v}^*_{\boldsymbol{k}} & \hat{u}_{\boldsymbol{k}} \end{pmatrix} \quad \text{and} \quad \hat{U}^\dagger_{\boldsymbol{k}}\hat{U}_{\boldsymbol{k}} = \mathbb{1} \end{aligned} \tag{19}$$

The matrices $\hat{u}_{\boldsymbol{k}}$ ($\hat{v}_{\boldsymbol{k}}$) are $N \times N$ matrices which describe the particle (hole) amplitudes of the Bogoliubov quasiparticles $\gamma_{\boldsymbol{k}}$ with energies $\pm E_{\boldsymbol{k}}$. To this end, $\hat{E}_{\boldsymbol{k}}$ denotes the corresponding diagonal matrix containing the particle-hole symmetric energy eigenvalues. The Bogoliubov quasiparticles are defined as

$$\begin{pmatrix} \gamma_{\boldsymbol{k},\uparrow} \\ \gamma^\dagger_{-\boldsymbol{k},\downarrow} \end{pmatrix} = \begin{pmatrix} \hat{u}_{\boldsymbol{k}} & \hat{v}_{\boldsymbol{k}} \\ -\hat{v}^*_{\boldsymbol{k}} & \hat{u}_{\boldsymbol{k}} \end{pmatrix} \begin{pmatrix} c_{\boldsymbol{k},\uparrow} \\ c^\dagger_{-\boldsymbol{k},\downarrow} \end{pmatrix}. \tag{20}$$

Together with Eq. (17), this yields a set of equations that needs to be solved self-consistently

$$\begin{aligned} \mathsf{H}_{\mathrm{MF}} &= \sum_{\boldsymbol{k}} \psi^\dagger_{\boldsymbol{k}} \begin{pmatrix} \hat{H}(\boldsymbol{k}) & \hat{\Delta}(\boldsymbol{k}) \\ \hat{\Delta}^\dagger(\boldsymbol{k}) & -\hat{H}(-\boldsymbol{k}) \end{pmatrix} \psi_{\boldsymbol{k}} + \mathrm{const.} \\ \langle c_{i\uparrow}(\boldsymbol{k})c_{j\downarrow}(-\boldsymbol{k}) - c_{i\downarrow}(\boldsymbol{k})c_{j\uparrow}(-\boldsymbol{k})\rangle_{\mathrm{MF}} &= \sum_n \left(u_{ni,\boldsymbol{k}}v^*_{nj,\boldsymbol{k}} + v_{nj,\boldsymbol{k}}u^*_{ni,\boldsymbol{k}}\right) \tanh\left(\frac{E_{n,\boldsymbol{k}}}{2T}\right) \end{aligned} \tag{21}$$

Here, $\sum_n$ denotes a sum over the positive quasiparticle energies $E_{n,\boldsymbol{k}} > 0$. To solve these non-linear equations self-consistently, we start with an initial guess respecting the symmetry of the gap parameter $\hat{\Delta}^{\mathrm{init}}_{ij}$ and iterate until convergence is achieved using a linear mixing $\hat{\Delta}^{n+1} = (1-\alpha)\hat{\Delta}^n - \alpha\hat{\Delta}^{n-1}$ scheme to avoid bipartite solutions in the fixed point iteration. In all of our calculations, we set the relative error for convergence to $\epsilon = 10^{-6}$ and set the mixing parameter to $\alpha = 0.2$.

In the manuscript, we only account for the gap parameter $\hat{\Delta}$ at the $\Gamma$-point of the Brillouin zone. This approximation may not change the underlying physics drastically as our microscopic interaction $\hat{\Gamma}_2$ in the static, long-wavelength limit ($q \to 0$) carries no momentum dependence and the size of the Brilluoin zone of MATTG is drastically reduced due to the large real-space unit cell. Hence, the $\boldsymbol{k}$-sum in Eq. (21) does not couple order parameters at different momentum points, but rather corresponds to a momentum average. Still, we checked that our results do not change qualitatively when taking a dense mesh with up to 24 $\boldsymbol{k}$-points in the BZ into account.

The full non-linear gap equation Eq. (21) is equivalent to minimizing the free energy of the system with respect to the pairing order parameter $\partial F/\partial\Delta_{ij} = 0$. To make sure that the superconducting state globally minimizes the free energy (and does not converge into possible local minima) we track the free energy for different initial guesses $\Delta^{\mathrm{init}}_{ij}$. The full expression of the free energy reads

$$F = E - TS = \sum_{n,\boldsymbol{k}} E_{n,\boldsymbol{k}} n_F\left(E_{n,\boldsymbol{k}}\right) - \sum_{n,\boldsymbol{k}} \left\{E_{n,\boldsymbol{k}} - \epsilon_{n,\boldsymbol{k}}\right\} - \sum_{\boldsymbol{k},ij} \frac{\Delta_{ij}(\boldsymbol{k})}{\Gamma_{2,ij}} - TS, \tag{22}$$

where $\epsilon_{n,\boldsymbol{k}}$ are the energies of the normal state Hamiltonian $H_0$ and the sum over $n$ runs over all positive quasiparticle energy states $E_{n,\boldsymbol{k}} > 0$. The entropy term of the free energy can be calculated using

$$S = -2\sum_{\boldsymbol{k},n} \Big\{ n_F\left[E_{n,\boldsymbol{k}}\right] \log\left(n_F\left[E_{n,\boldsymbol{k}}\right]\right) + \left(1 - n_F\left[E_{n,\boldsymbol{k}}\right]\right) \log\left(1 - n_F\left[E_{n,\boldsymbol{k}}\right]\right) \Big\}. \tag{23}$$

[1] X. Liang, Z. A. H. Goodwin, V. Vitale, F. Corsetti, A. A. Mostofi, and J. Lischner, Phys. Rev. B **102**, 155146 (2020).

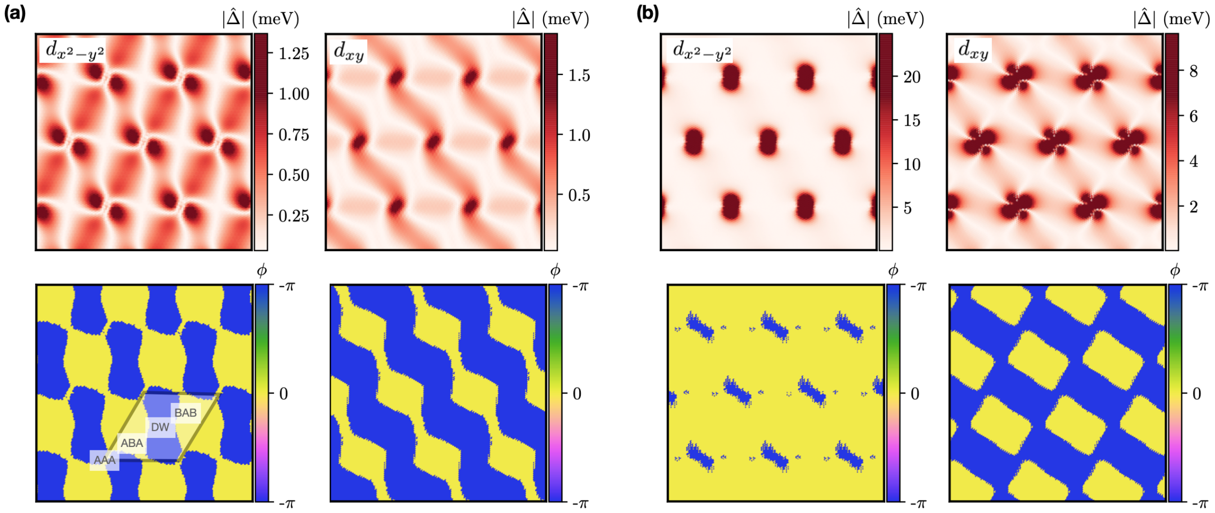


**Supplementary Figure** 15. **Atomistic nematic gap parameter $\hat{\Delta}$ in MATTG. (a)** Amplitude and phase distribution of the superconducting order parameter $\hat{\Delta}$ in the outer layer of MATTG projected onto the two local $d$-wave components for $\nu = -2.5$, $T = 0.2\,\mathrm{K}$. The order parameter is real-valued such that the phase consists of domains separated by $\pi$ (blue and yellow color coding). The amplitude is strongly enhanced in the AAA regions and the order parameter breaks the original $C_3$ symmetry of the normal-state Hamiltonian. **(b)** The amplitude in the middle layer is enhanced by a factor of $\sim 10$. Compared to the upper (lower) layer the phase is shifted by $\pi$ as a result of the original interlayer repulsion in the tight-binding Hamiltonian.

[2] A. Lopez-Bezanilla and J. L. Lado, Phys. Rev. Research **2**, 033357 (2020).
[3] Z. A. Goodwin, V. Vitale, X. Liang, A. A. Mostofi, and J. Lischner, Electronic Structure **2**, 034001 (2020).
[4] L. Rademaker, D. A. Abanin, and P. Mellado, Phys. Rev. B **100**, 205114 (2019).
[5] T. Cea, N. R. Walet, and F. Guinea, Phys. Rev. B **100**, 205113 (2019).
[6] F. Guinea and N. R. Walet, PNAS **115**, 13174–13179 (2018).
[7] M. Calderón and E. Bascones, Phys. Rev. B **102**, 155149 (2020).
[8] T. O. Wehling, E. Şaşıoğlu, C. Friedrich, A. I. Lichtenstein, M. I. Katsnelson, and S. Blügel, Phys. Rev. Lett. **106**, 236805 (2011).
[9] E. Khalaf, A. J. Kruchkov, G. Tarnopolsky, and A. Vishwanath, Phys. Rev. B **100**, 085109 (2019).
[10] L. Klebl, Z. A. H. Goodwin, A. A. Mostofi, D. M. Kennes, and J. Lischner, Phys. Rev. B **103**, 195127 (2021).
[11] E. J. G. Santos and E. Kaxiras, Nano Lett. **13**, 898 (2013).
[12] J. M. Park, Y. Cao, K. Watanabe, T. Taniguchi, and P. Jarillo-Herrero, Nature **590**, 249 (2021).
[13] L. Klebl and C. Honerkamp, Physical Review B **100**, 155145 (2019).
[14] H. Q. Lin and J. E. Hirsch, Phys. Rev. B **35**, 3359 (1987).
[15] N. F. Berk and J. R. Schrieffer, Phys. Rev. Lett. **17**, 433 (1966).
